# Supplementary material for: Bubble propagation on a rail: a concept for sorting bubbles by size
Source: arXiv:1712.01623 source file (2017-12-05)
Supplement: Supplementary file 1 [file SupplementaryMaterial_Franco-Gomez-et-al.pdf]

# Supplementary Material

## Bubble propagation on a rail: a concept for sorting bubbles by size

Andrés Franco-Gómez,<sup>a</sup> Alice B. Thompson,<sup>b</sup> Andrew L. Hazel<sup>b</sup> and Anne Juel<sup>\*a</sup>

<sup>a</sup> Manchester Centre for Nonlinear Dynamics & School of Physics & Astronomy, The University of Manchester, Manchester M13 9PL, UK. Tel: 0161 2754071; E-mail: anne.juel@manchester.ac.uk

<sup>b</sup> Manchester Centre for Nonlinear Dynamics & School of Mathematics, The University of Manchester, Manchester M13 9PL, UK.

### 1 Experimental methods

#### 1.1 Ensuring a constant bubble volume during experimentation

Bubbles that were in equilibrium in the absence of flow were observed to gain (lose) volume through diffusion of air across the oil-air interface. This is due to pressure changes in the oil which alter the solubility of air in oil, when bubbles propagate under low (high) imposed flow rate, respectively. In order to ensure that the bubble retained a constant volume during experimentation, the silicone oil filling the channel (200 ml) was saturated with air prior to experimentation, by pumping air into the liquid for 30 min using an aquarium air pump (HAILEA ACO-9601) at a flow rate of 3.2 L/min and pressure  $> 0.012$  MPa. In addition, the infusion flow rate applied to return the bubble to the inlet between experiments was optimised to ensure minimal volume variations with  $Q^* = 15.5$  ml/min and  $Q^* = 9.0$  ml/min for the rails of widths  $w^* = 6.9$  mm and 10.7 mm, respectively. As a result, the projected area of bubbles before and after each experiment remained constant to within  $\delta A = \pm 1$  % for  $Q^* \leq 30$  ml/min. However, this increased to  $2 \leq \delta A \leq 10$  % for larger flow rates  $30 < Q^* \leq 50$  ml/min.

#### 1.2 Measurement of the rail profile

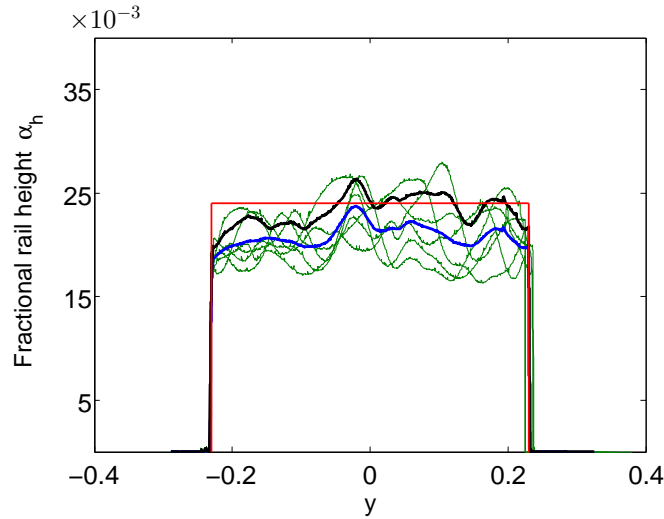

**Fig. S.1** Experimental rail profile measured with profilometry (DekTak IIA, resolution 30 nm) at 6 positions along the length of the rail (green lines). The experimental profiles demonstrate that the rail has approximately vertical side walls. The blue line corresponds to the point by point average of the 6 profiles, with an overall average height of  $\langle h^* \rangle = 20.91 \mu\text{m}$  and a standard deviation of  $\sigma^* = 2.4 \mu\text{m}$ . The black solid line denotes the point-by-point average profile augmented by one standard deviation, with an overall average height of  $\langle h^* \rangle + \sigma^* = 23.32 \mu\text{m}$ . This value is consistent with the height measured with a micrometer (Mitutoyo IP65) of  $h_{mic}^* = 24 \pm 1 \mu\text{m}$ , which corresponds to the profile plotted with a red line.

The experimental rail profile was measured with profilometry (DekTak IIA, resolution  $0.1 \mu\text{m}$ ) at 6 positions along the length of the rail as shown in Figure S.1. The experimental profiles demonstrate that the rail has approximately vertical side walls. The overall

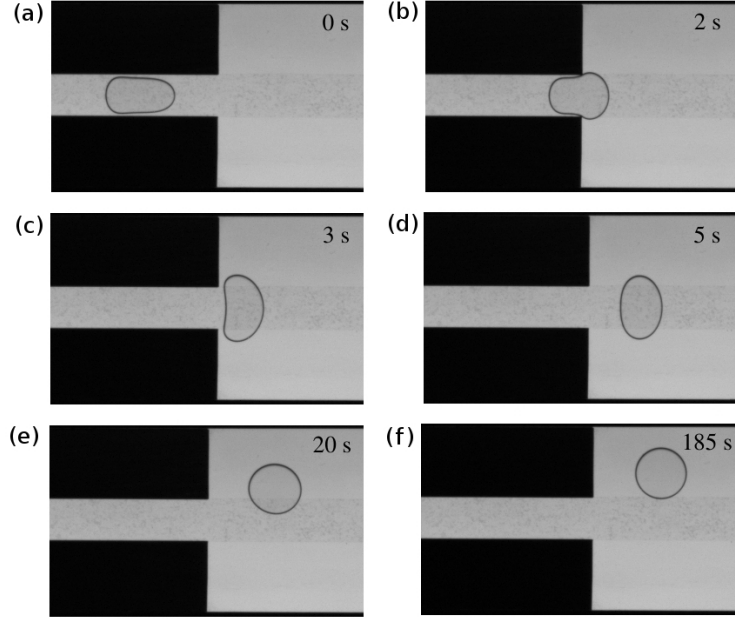

**Fig. S.2** Experimental protocol used to impose the initial position of the bubble. (a) A bubble is propagated in a guiding channel which spans the width of the rail at a small flow rate of  $Q^* = 1.5$  ml/min. (b–c) The bubble is released in a centred position into the main channel and allowed to travel over a distance of approximately 15 mm in order for its shape to relax. (d) The flow is interrupted by setting  $Q^* = 0$  ml/min for less than five seconds before a constant flow rate is imposed, during which the bubble remains centred over the thin rail. This is the symmetric on-rail initial condition. (e) If  $Q^* = 0$  is maintained beyond a few seconds, the bubble spontaneously migrates to an off-centred position, and a constant flow rate is imposed after 20 s. A preferred direction of migration is typically set by a small systematic bias in the experiment. This is the off-rail initial condition. (f) By maintaining  $Q^* = 0$ , the bubble eventually reaches a stable static off-rail position.

average height augmented by one standard deviation,  $\langle h^* \rangle + \sigma^* = 23.32 \mu\text{m}$ , is consistent with the height measured with a micrometer (Mitutoyo IP65) of  $h_{mic}^* = 24 \pm 1 \mu\text{m}$ .

### 1.3 Setting the initial conditions for bubble propagation.

The protocol employed to place bubbles either on or off the rail prior to experimentation is illustrated in Figure S.2. The bubble was confined to a channel that spanned the width of the rail upstream of the flow channel. It was propagated at a low flow rate of  $Q^* = 1.5$  ml/min along this guiding channel and then beyond the sudden expansion to the flow channel by approximately 15 mm in order to allow its shape to relax. Interrupting the flow for up to 5 s before a constant flow rate was imposed led to an on-rail initial condition, while longer waiting times of 20 s allowed spontaneous migration of the bubble to an off-centred position, so that the bubble was off-rail when the flow was subsequently imposed.

### 1.4 Measurement of the thin films separating the bubble from the top and bottom boundaries.

The average thickness of the fluid films separating the bubble from the top and bottom boundaries of the channel can be estimated by monitoring the change in projected area (or effective diameter) when the bubble is in motion compared to when it is at rest. In particular, assuming that the bubble volume is constant, an increase in observed diameter when in motion corresponds to an average thickening of the films with flow rate.

The effective diameter  $D^*$  is obtained from the observed bubble area  $A^*$  using  $D^* = 2\sqrt{A^*/\pi}$ . For both on-rail and off-rail propagation modes, we find that the ratio of the diameter of a bubble at flow rate  $Q^*$  to its static diameter increases approximately linearly as a function of flow rate as shown in Figure S.3. Note that as there is no stable on-rail state at  $Q = 0$ ,  $D_0^*$  is measured in the static off-rail state throughout this section. The data for different bubble sizes spanning the experimental range collapse approximately onto a master curve, suggesting that film thicknesses are independent of bubble size within this range. In both configurations, the diameter increases

by 33% from  $Q = 0$  to  $Q = 6.6 \times 10^{-2}$  ( $Q^* = 50$  ml/min). The scatter in the data increases marginally for  $Q > 4.0 \times 10^{-2}$  ( $Q^* > 30$  ml/min). This is the result of increased volume variations of the bubble from  $\pm 1\%$  for  $Q^* \leq 30$  ml/min up to  $\pm 5\%$  for  $Q^* = 50$  ml/min.

In order to obtain an estimate of the film thickness from observed diameters, we assume that the bubble volume is conserved between motion and rest, and approximate its shape by a cylinder. We suppose that the films above and below the bubble each have thickness  $t_0^*$  when static, and  $t_Q^*$  when in motion. The air bubble occupies the remaining height in the channel. Requiring that these two cylindrical bubbles have equal volume implies

$$V^* = \frac{\pi(D_0^*)^2}{4}(H^* - 2t_0^*) = \frac{\pi(D_Q^*)^2}{4}(H^* - 2t_Q^*), \quad (\text{S.1})$$

where  $H^*$  is the total channel height. We rearrange this to give

$$t_Q^* = \frac{1}{2} \left[ 1 - \left( \frac{D_0^*}{D_Q^*} \right)^2 \right] + t_0^* \left( \frac{D_0^*}{D_Q^*} \right)^2. \quad (\text{S.2})$$

This equation has two important consequences: an increase in effective diameter so that  $D_Q^* > D_0^*$  corresponds to an increase in film thickness, and increasing the static film thickness  $t_0^*$  (expected to be vanishingly small) for the same observed static diameter  $D_0^*$  further increases the dynamic film thickness. However, we must recall this is only a statement about average thickness, and neglects the presence of the obstacle. The obstacle occupies 2.4% of the channel height, so would be expected to increase the static diameter by around 1% for a bubble that is entirely over the obstacle. As  $Q$  increases, the observed changes in diameter rapidly surpass this level.

Estimated values for the film thickness using (S.2) with  $t_0^* \sim 0$  are given in Table S.1 for on-rail and off-rail propagating bubbles, respectively. These values are computed within the range of volume change of  $\pm 1\%$ . The estimates do not show significant differences between on-rail and off-rail propagation, however, both on-rail and off-rail bubbles usually partially overlap the obstacle. The fluid film thickness for  $Q = 2.5 \times 10^{-2}$  ( $Q^* = 19$  ml/min), which is the maximum flow rate in the stability diagram of Figure 7a, is approximately 4 times larger than the height of the rail, which suggests that the bubble interface feels a much smoother obstacle than the sharp edges shown in Figure S.1.

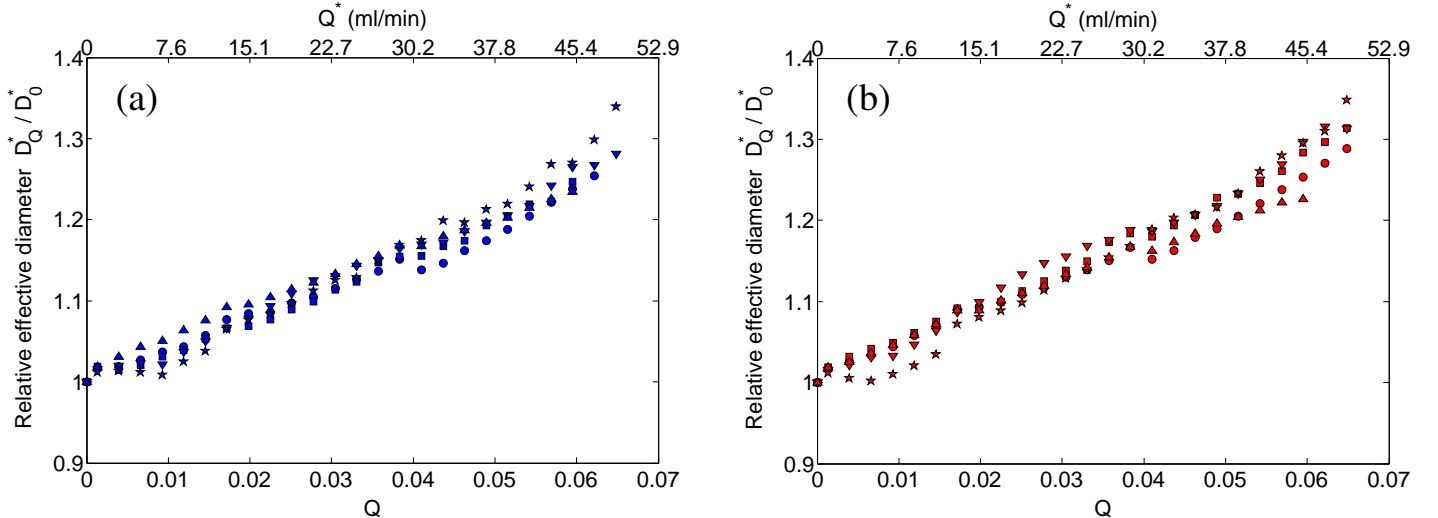

**Fig. S.3** Relative bubble diameter  $D_R = D_Q^*/D_0^*$ , where  $D_Q^*$  is the diameter of a bubble propagating under flow rate  $Q$  and  $D_0^*$  is its static diameter, as a function of the nondimensional flow rate  $Q$  (dimensional flow rate  $Q^*$  in ml/min): (a) off-rail initial condition; (b) on-rail initial condition. The different symbols correspond to (★)  $D_0^* = 5.3 \pm 0.2$  mm, (▼)  $7.2 \pm 0.5$  mm, (●)  $9.2 \pm 0.5$  mm, (■)  $11.4 \pm 1.0$  mm and (▲)  $12.5 \pm 1.5$  mm. The bubble diameter is controlled so that it varies by  $\delta D = \pm 0.5\%$  for flow rates  $Q < 4.0 \times 10^{-2}$  ( $Q^* < 30$  ml/min), and  $\delta D = 5\%$  for  $Q > 4.0 \times 10^{-2}$  ( $Q^* > 30$  ml/min). The bubble diameter increases by 18% when the flow rate is increased from  $Q = 0$  to  $Q = 3.8 \times 10^{-2}$  ( $Q^* = 29$  ml/min).

## 2 Numerical Implementation

The equation (2), boundary conditions (3–5) and the volume constraint (6) in the main text are discretised using a finite element method and the corresponding discrete residuals are assembled and solved using the library `oomph-lib`<sup>1</sup>. The methods are essentially the

**Table S.1** Estimate of average fluid film thickness for a bubble propagating either off-rail or on-rail.

| Bubble static diameter $D_0^*$<br>(mm) | Off-rail          | film thickness<br>at $Q = 2.5 \times 10^{-2}$<br>( $Q^* = 19$ ml/min) | film thickness<br>at $Q = 3.8 \times 10^{-2}$<br>( $Q^* = 29$ ml/min) | On-rail           | film thickness<br>at $Q = 2.5 \times 10^{-2}$<br>( $Q^* = 19$ ml/min) | film thickness<br>at $Q = 3.8 \times 10^{-2}$<br>( $Q^* = 29$ ml/min) |
|----------------------------------------|-------------------|-----------------------------------------------------------------------|-----------------------------------------------------------------------|-------------------|-----------------------------------------------------------------------|-----------------------------------------------------------------------|
|                                        | ( $\mu\text{m}$ ) | ( $\mu\text{m}$ )                                                     | ( $\mu\text{m}$ )                                                     | ( $\mu\text{m}$ ) | ( $\mu\text{m}$ )                                                     | ( $\mu\text{m}$ )                                                     |
| 5.3                                    | 84                | 134                                                                   | 85                                                                    | 133               |                                                                       |                                                                       |
| 7.2                                    | 94                | 131                                                                   | 111                                                                   | 146               |                                                                       |                                                                       |
| 9.2                                    | 84                | 123                                                                   | 94                                                                    | 133               |                                                                       |                                                                       |
| 11.4                                   | 78                | 125                                                                   | 96                                                                    | 143               |                                                                       |                                                                       |
| 12.5                                   | 97                | 133                                                                   | 95                                                                    | 133               |                                                                       |                                                                       |

same as those used and validated in Thompson *et al.* (2014)<sup>2</sup> and Franco-Gomez *et al.* (2016)<sup>3</sup>. In summary, we use a boundary-fitted moving mesh method: the mesh is modified in response to changes in the bubble size and shape. These methods typically have better mass conservation properties than immersed interface methods. An isoparametric Galerkin method is used to solve the weak form of equation (2):

$$\int_{\Omega} b^3(y) \nabla p \cdot \nabla \psi d\Omega = \int_{\partial\Omega} \psi b^3(y) \hat{\mathbf{n}} \cdot \nabla p ds, \quad (\text{S.3})$$

where  $\psi$  represents piecewise quadratic test functions that are also used to interpolate the fluid pressure and unknown nodal positions. The boundary conditions (3) and (5) give conditions for  $\hat{\mathbf{n}} \cdot \nabla p$  or  $p$  on each boundary of the fluid domain. The pressure gradient conditions are used directly in the right-hand side of equation (S.3). The pressure boundary conditions are imposed by fixing the appropriate pressure unknowns and removing the corresponding discrete residuals from the system.

The fluid domain is discretised via triangular elements and mesh updates are handled by treating the mesh as a pseudo-elastic body. The required bubble deformation is enforced by applying a normal stress to the mesh equations at the bubble surface, determined by the weak form of the dynamic boundary condition (4). The curvature term is not smooth for a piecewise quadratic representation of the interface, and we obtain a continuous curvature term by projecting a weak derivative of the boundary tangent vector onto a piecewise quadratic space.

The volume constraint (6) is converted into a line integral via the divergence theorem

$$\oint_{\partial\Omega_b} x b(y) n_x ds = V_0, \quad (\text{S.4})$$

where  $n_x$  is the  $x$ -component of the normal to the interface. The constraint on the bubble centroid is also computed via a surface line integral

$$\oint_{\partial\Omega_b} x^2 b(y) n_x ds = 0, \quad (\text{S.5})$$

In the model, the centroid offset  $y_c$  is calculated using a height-weighted average:

$$y_c = \frac{\oint_{\partial\Omega_b} x y b(y) n_x ds}{V_0}. \quad (\text{S.6})$$

The line integrals (S.4), (S.5) and (S.6) are then assembled at the same time as the contributions to the dynamic and kinematic boundary conditions. The experimental results for  $y_c$  do not include the height-weighting; the two definitions differ by at most 1.1%, which is within the experimental margin of error.

Steady solutions are computed using Newton's method combined with arc-length continuation steps. The implicit second order BDF2 method is used for unsteady calculations and the eigenproblem associated with a linear stability analysis formulated by Thompson *et al.*<sup>2</sup> is solved using a Block Krylov Schur iterative algorithm.

As the system parameters change, elements within the bulk mesh can become distorted. We perform a complete remesh when selected tolerances are exceeded by either a 'Z2' estimate of the error based on continuity of  $-b^2 \nabla p$  between bulk elements or the curvature of the interface. The fluid domain was typically discretised with around 3000 triangular elements and we confirmed that further refinement of the mesh to 10000 elements did not change the results to graphical accuracy.

## References

- [1] M. Heil and A. L. Hazel, *Lecture Notes on Computational Science and Engineering*, 2006, **53**, 19–49.
- [2] A. B. Thompson, A. Juel and A. L. Hazel, *J. Fluid Mech.*, 2014, **746**, 123–164.
- [3] A. Franco-Gómez, A. B. Thompson, A. L. Hazel and A. Juel, *J. Fluid Mech.*, 2016, **794**, 343–368.
